# Supplementary material for: Assessing the quantumness of the annealing dynamics via Leggett Gargs inequalities: a weak measurement approach
Source: arXiv:1902.08257 ancillary file (2019-02-21)
Supplement: Supplementary file 1 [file SupMaterials_v4.pdf]

# Leggett and Garg's inequalities and quantum annealing: Supplementary Information

V. Vitale,<sup>1</sup> G. De Filippis,<sup>1,2</sup> A. De Candia,<sup>1</sup> A. Tagliacozzo,<sup>1,2</sup> V. Cataudella,<sup>1,2</sup> and P. Lucignano<sup>2,1</sup>

<sup>1</sup>*Dipartimento di Fisica "Ettore Pancini", Università di Napoli "Federico II", Monte S. Angelo, I-80126 Napoli, Italy*

<sup>2</sup>*CNR-SPIN, Monte S. Angelo via Cinthia, I-80126 Napoli, Italy*

(Dated: December 27, 2018)

## I. LINDBLAD EQUATION

In this Section we recall the quantum dynamics of an open quantum system described by the time dependent Hamiltonian  $H_S([A_\alpha], t)$ , interacting with an ohmic thermal bath in the weak coupling Lindblad approach.  $[A_\alpha]$  are a set of Hermitian and dimensionless operators of the system while the bath is described by the Hermitian Hamiltonian  $H_B([B_\nu])$ , where  $[B_\nu]$  are operator describing the bath. Let  $U_S$  and  $U_B$  be the time evolution operators of the system and bath only:

$$U_S(t, t') = \mathcal{T} e^{-i \int_{t'}^t H_S(\tau) d\tau}; \quad (1)$$

$$U_B(t, t') = e^{-i H_B(t-t')}. \quad (2)$$

Here  $\mathcal{T}$  is the time ordering operator in real time. The evolution of the system and the bath in the absence of interaction is governed by

$$U_0(t, t') = U_S(t, t') \otimes U_B(t, t'). \quad (3)$$

The interaction between system and bath is described, in full generality, by

$$H_I = \sum_{\alpha} g_{\alpha} A_{\alpha} \otimes B_{\alpha}, \quad (4)$$

where  $g_{\alpha}$  are coupling constants. Adiabatic switching of the interaction at negative times is assumed. We define the total Hamiltonian for the joint system-bath universe,

$$H(t) = H_S(t) + H_B + H_I, \quad (5)$$

and the time-dependent density operator  $\rho(t)$ , whose dynamics is expressed by the Von Neumann equation and the full system-bath evolution operator,

$$U(t, t') = \mathcal{T} e^{-i \int_{t'}^t H(\tau) d\tau}. \quad (6)$$

Moving to the interaction picture, we define

$$\tilde{U}(t, 0) = U_0^{\dagger}(t, 0) U(t, 0), \quad (7a)$$

$$\tilde{\rho}(t) = U_0^{\dagger}(t, 0) \rho(t) U_0(t, 0), \quad (7b)$$

$$\tilde{H}_I(t) = U_0^{\dagger}(t, 0) H_I(t) U_0(t, 0), \quad (7c)$$

where

$$\tilde{H}_I(t) = U_0^{\dagger}(t, 0) H_I U_0(t, 0) = g \sum_{\alpha} A_{\alpha}(t) \otimes B_{\alpha}(t), \quad (8)$$

and  $A_{\alpha}(t)$ ,  $B_{\alpha}(t)$  are the time-evolved operators,

$$A_{\alpha}(t) = U_S^{\dagger}(t, 0) A_{\alpha} U_S(t, 0), \quad (9)$$

$$B_{\alpha}(t) = U_B^{\dagger}(t, 0) B_{\alpha} U_B(t, 0). \quad (10)$$

$\tilde{U}(t, 0)$  and  $\tilde{\rho}(t)$  satisfy the following differential equations:

$$\begin{cases} \frac{d}{dt} \tilde{U}(t, 0) = -i \tilde{H}_I(t) \tilde{U}(t, 0), \\ \tilde{U}(0, 0) = \mathbb{I}, \end{cases} \quad (11a)$$

$$\begin{cases} \frac{d}{dt} \tilde{\rho}(t) = -i [\tilde{H}_I(t), \tilde{\rho}(t)], \\ \tilde{\rho}(0) = \mathbb{I}. \end{cases} \quad (11b)$$

Given the two point correlation function  $\mathcal{B}_{\alpha\beta}(\tau) \equiv \langle B_{\alpha}(\tau) B_{\beta}(0) \rangle$ , the spectral-density matrix of the bath is:

$$\Gamma_{\alpha\beta}(\omega) \equiv \int_0^{\infty} d\tau e^{i\omega\tau} \mathcal{B}_{\alpha\beta}(\tau) = \frac{1}{2} \gamma_{\alpha\beta}(\omega) + i S_{\alpha\beta}(\omega), \quad (12)$$

where its real and imaginary part are

$$\gamma_{\alpha\beta}(\omega) = \int_{-\infty}^{\infty} d\tau e^{i\omega\tau} \mathcal{B}_{\alpha\beta}(\tau) = \gamma_{\alpha\beta}^*(\omega), \quad (13a)$$

$$S_{\alpha\beta}(\omega) = \int_{-\infty}^{\infty} \frac{d\omega'}{2\pi} \gamma_{\alpha\beta}(\omega') P\left(\frac{1}{\omega - \omega'}\right) = S_{\alpha\beta}^*(\omega). \quad (13b)$$

Lindblad theory eventually leads to master equation for the reduced density matrix (representing only the system variables),

$$\frac{d\rho_Q(t)}{dt} = -i [H(t) + H_{LS}(t), \rho(t)] + \mathcal{D}[\rho_Q(t)], \quad (14)$$

where the adiabatic dissipator  $\mathcal{D}$  is

$$\mathcal{D}[\rho_Q(t)] = \sum_{\alpha\beta} \sum_{\omega} \gamma_{\alpha\beta}(\omega) \left[ L_{\beta\omega}(t) \rho_Q(t) L_{\alpha\omega}^\dagger(t) - \frac{1}{2} \{ L_{\alpha\omega}^\dagger(t) L_{\beta\omega}(t), \rho_Q(t) \} \right] \quad (15)$$

and the Lamb shift Hamiltonian takes the form

$$H_{\text{LS}}(t) = \sum_{\alpha\beta} \sum_{\omega} S_{\alpha\beta}(\omega) L_{\alpha\omega}^\dagger(t) L_{\beta\omega}(t). \quad (16)$$

They are written in terms of the Lindblad operators  $L_{\alpha\omega}(t)$ , which are defined as

$$L_{\alpha\omega}(t) = \sum_{\epsilon_a(t) - \epsilon_b(t) = \omega} |\epsilon_a(t)\rangle \langle \epsilon_a(t)| A_\alpha |\epsilon_b(t)\rangle \langle \epsilon_b(t)|, \quad (17)$$

where  $\{\epsilon_a(t)\}$  are the instantaneous eigenvectors of the system Hamiltonian.

The universe we study here is a single spin coupled to a bath of bosonic harmonic oscillators described by the Hamiltonian

$$H_B = \sum_{k=1}^{\infty} \omega_k b_k^\dagger b_k, \quad (18)$$

where  $b_k^\dagger$  and  $b_k$  are, respectively raising and lowering operators for the  $k$ -th oscillator with frequency  $\omega_k$  and the frequency spectrum is assumed to be continuous as usually in the spin-boson model<sup>1-3</sup>. The bath is assumed to be in thermal equilibrium at inverse temperature  $\beta = 1/k_B T$ , so that its density operator is just  $\rho_B = e^{-\beta H_B} / \mathcal{Z}$ .

The interaction between the system and the bath is  $H_I = \sigma_z \otimes B$ , where the operator  $B$  is defined  $B = \sum_k g_k (b_k^\dagger + b_k)$ .

The Fourier transform of the bath correlation function is:

$$\gamma(\omega) = \frac{2\pi J(|\omega|)}{1 - e^{-\beta|\omega|}} g^2 \left( \Theta(\omega) + e^{-\beta|\omega|} \Theta(-\omega) \right), \quad (19)$$

where  $\Theta(\pm\omega)$  are Heaviside functions<sup>1</sup>. The model is fully determined once the explicit form of the function  $J(\omega)$  is given. In this paper, we consider an Ohmic bath<sup>2</sup>, characterized by

$$J(\omega) = \eta \frac{\omega^\nu}{\omega_c^{\nu-1}} e^{-\omega/\omega_c}, \quad \text{with } \nu = 1, \quad (20)$$

where  $\omega_c$  is a high-frequency cut-off that is the maximum phonon energy and  $\eta$  is a dimensional parameter with dimensions of time squared. In conclusion, we define  $\alpha = \eta g^2$  and explicit  $\gamma$  as follows:

$$\gamma(\omega) = 2\pi\alpha \frac{\omega e^{-|\omega|/\omega_c}}{1 - e^{-\beta\omega}}, \quad (21)$$

## II. LEGGETT-GARG'S INEQUALITIES

The starting point of the Leggett-Garg's Inequalities is a definition of macrorealism as a principle one wants to stick at ("is the flux there when nobody looks?"). This is contained in a small set of principles or assumptions that, quoting directly from<sup>4</sup>, reads:

**A: Macroscopic realism per se.** A macroscopic object which has available to it two or more macroscopically distinct states is, at any given time, in a definite one of those states.

**B: Non-invasive measurability.** It is possible in principle to determine which of these states the system is in, without any effect on the state itself or on the subsequent system dynamics.

**C: Induction.** The properties of ensembles are determined exclusively by initial conditions (and in particular not by final conditions).

These properties define what has been called "classicality" or "macrorealism".

Based on the assumptions above, Leggett and Garg derived Bell's-like inequalities that any system behaving classically should obey<sup>5</sup>. Violations of these inequalities provide evidence of quantum behavior of a system if one accepts that the alternative to classical probabilities is quantum mechanics. Therefore these violations can be interpreted as an indicator of the "quantumness" of a system.

Following Ref.<sup>6</sup>, in this section we briefly introduce the Leggett-Garg's inequalities and discuss their properties as witness of "quantumness".

Let us begin with the definition of a classical dichotomic variable  $Q$  which can assume value  $+1$  or  $-1$ :  $Q(t_i) = Q_i$  stands for the measurement value of the observable at time  $t_i$ . We denote with  $P_i(Q_i)$  the probability of obtaining the result  $Q_i$  at time  $t_i$ . The correlation function  $C_{i,j}$  can be defined as follows:

$$C_{i,j} = \sum_{Q_i, Q_j = \pm 1} Q_i Q_j P_{ij}(Q_i, Q_j) = \langle Q_i Q_j \rangle, \quad (22)$$

where the subscripts of  $P$  remind us of the times at which the measurements were performed. Assumption A, that is "Macrorealism per se", guarantees that  $P_{ij}$  can be obtained as the marginal probability of  $P_{ijk}(Q_i, Q_j, Q_k)$ .

$$P_{ij}(Q_i, Q_j) = \sum_{Q_k; t_k \neq t_i, t_j} P_{ijk}(Q_i, Q_j, Q_k) \quad (23)$$

The assumption of "Non-invasive measurability" allows to drop the subscripts of  $P_{ijk}$  and use the  $P(Q_i, Q_j, Q_k)$

alone (with  $\sum_{Q_i, Q_j, Q_k} P_{ijk}(Q_i, Q_j, Q_k) = 1$ ) to calculate the three correlation functions:  $C_{1,2}, C_{2,3}, C_{1,3}$ . We obtain

$$\begin{aligned}
C_{1,2} &= P(+, +, +) + P(+, +, -) - P(-, +, -) + \\
&\quad + P(-, -, +) + P(-, -, -) - P(+, -, +) + \\
&\quad - P(+, -, -) - P(-, +, +), \\
C_{1,3} &= P(+, +, +) + P(+, -, +) - P(-, -, +) + \\
&\quad + P(-, +, -) + P(-, -, -) - P(+, +, -) + \\
&\quad - P(+, -, -) - P(-, +, +), \\
C_{2,3} &= P(+, +, +) + P(-, +, +) - P(-, -, +) + \\
&\quad + P(+, -, -) + P(-, -, -) - P(+, +, -) + \\
&\quad - P(-, +, +) - P(+, -, +),
\end{aligned} \tag{24}$$

where  $\pm$  stands for  $Q = \pm$ . Next, we define

$$K_3^a = C_{1,2} + C_{2,3} - C_{1,3} = 1 - 4[P(+, -, +) + P(-, +, -)]. \tag{25}$$

The upper bound of  $K_3^a$  corresponds to  $P(+, -, +) = P(-, +, -) = 0$ , giving  $K_3^a = 1$ ; the lower bound, instead,  $K_3^a \geq -3$  corresponds to  $P(+, -, +) + P(-, +, -) = 1$ . Besides the inequality

$$-3 \leq K_3 \leq 1 \tag{26}$$

other inequalities exist, that can be found in the literature.

Various symmetry properties can be used to derive other constraints on the correlations. The change  $Q \rightarrow -Q$  in  $K_3^a$  gives rise to the following inequality:

$$-3 \leq K_3^b \leq 1; \quad K_3^b \equiv -C_{1,2} - C_{2,3} - C_{1,3}. \tag{27}$$

Finally, the last, different, third order inequality can be obtained from  $K_3^a$ , just changing a sign:

$$-3 \leq K_3^c \leq 1; \quad K_3^c \equiv -C_{1,2} + C_{2,3} + C_{1,3}. \tag{28}$$

These are the only three different inequalities that can be derived from correlations to third order. Higher order inequalities can also be constructed.

### III. MEASUREMENT SCHEME

In this Section we sketch an idealized measurement approach which can be extended from projective to weak measurement, to reduce the invasiveness of the classical measurement process. Resorting to a weak measurement scheme is unavoidable to allow for a successful annealing. Indeed in Fig. 1 we show the residual energy and the ground state population during the annealing dynamics in the absence and in the presence of two projective measurements in order to demonstrate the necessity of weakening the measurement approach. In the panels a) and c) we show the residual energy and the ground state population in the absence of measurements. At the annealing time the latter is approximately 1 and the former

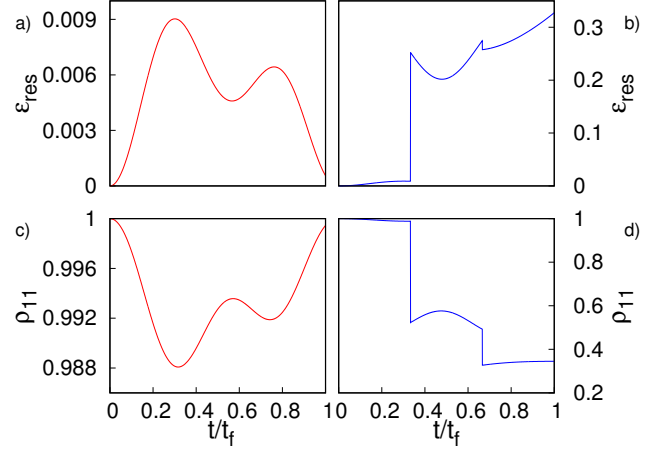

FIG. 1. Residual Energy and ground state population (Fidelity) as a function of  $t/t_f$  ( $t_f = 10\sqrt{2}$ ). a) Residual Energy in the absence of measurements; b) Residual Energy in the case of measurements at times  $t_2 = 0.3 t/t_f$  and  $t_3 = 0.6 t/t_f$ ; c) Fidelity in absence of measurements; d) Fidelity in the case of measurements at times  $t_2 = 0.3 t/t_f$  and  $t_3 = 0.6 t/t_f$

is nearly 0 which reveals that the quantum annealing has been successful. On the other hand, in the panels b) and d) we calculate the residual energy and the ground state population, while measuring one of the possible  $C_{2,3}$  necessary to build the  $K_3$ s. Clearly, at the measurement times  $t_2$  and  $t_3$ , the (projective) measurement procedure suddenly alters the population of the ground state. The ground state population is very poor at the annealing time, and the residual energy sizably larger than zero, signaling that the annealing procedure has failed. Thus approaching to the calculation of the Leggett-Garg's functions with weak measurements is necessary to evaluate the coherence of the system during the quantum annealing with negligible effects on the dynamics.

For the sake of concreteness, we consider a superconducting flux qubit, as the system S, and an hysteretic DC SQUID, as the ancilla/detector A (Fig. 2). In a superconducting flux qubit, when polarized by an external flux  $\phi$  close to  $\phi_0/2$ , where  $\phi_0$  is the flux quantum, the current can flow clockwise or anti-clockwise. A spin degree of freedom can be associated to the circulating current, e.g. the state of the system can be denoted by  $|\uparrow\rangle$ , if the current is clockwise, while it is  $|\downarrow\rangle$ , if the current is anti-clockwise.

On this basis of eigenstates of  $\sigma_z$ , the Hamiltonian of the flux qubit can be written as in the main text:

$$H_S = \frac{\Gamma_x}{2} \sigma_x + \frac{\Gamma_z}{2} \sigma_z, \tag{29}$$

where  $\Gamma_x$  is the tunnel coupling between the current states and  $\Gamma_z = 2I_p(\frac{\phi_0}{2} - \phi)$ , where  $I_p$  is the magnitude of the current flowing in the flux qubit.

By introducing a linear time dependence in the same

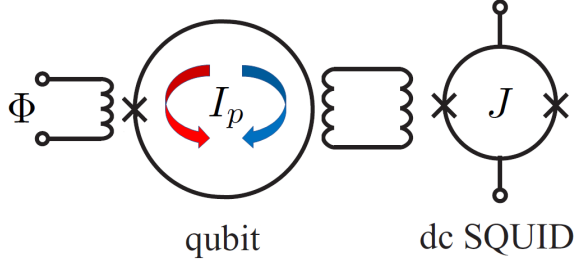

FIG. 2. Diagram of the superconducting flux qubit coupled to the hysteretic DC SQUID.

hamiltonian one obtains:

$$H(s) = (1-s)\frac{\Gamma_x}{2}\sigma_x + s\frac{\Gamma_z}{2}\sigma_z, \quad (30)$$

which is the Hamiltonian that describes a linear annealing protocol. Here  $s = t/t_f$  goes from 0 to 1 and  $t_f$  is the total annealing time. The system evolves along its dynamics and, to evaluate the possible violation of the Leggett-Garg's inequalities, it is necessary to measure correlations of system variables at different times.

The quantum state of the system can be read out by exploiting the mutual inductance  $M$  of the qubit with the ancilla DC SQUID, represented by the interaction Hamiltonian  $H_I = MJ I_p \sigma_z$ . Here  $J$  is the current circulating in the DC SQUID.

As described in ref.<sup>7</sup>, the measurement can be performed considering that the ancilla, appropriately polarized with  $J$  close to the critical current  $I_c$ , by means of a flux  $\Phi \sim n\phi_0$  ( $n$  integer), can be either in a superconducting state with zero voltage  $V = 0$  or in a dissipative state with a finite voltage  $\bar{V}$ .

Let the circulating current in A be  $J < I_c$ , prior to measurement. With a short current pulse  $I_b$ , the DC SQUID can be biased very close to its critical current  $I_c$ . During the pulse the ancilla has a certain probability of staying in the  $V = 0$  state, or switching to the dissipative state depending on the state of the qubit  $|\uparrow\rangle, |\downarrow\rangle$ . Indeed, the circulating current  $I_p$  induces an electromotive force in the A loop, which increases or decreases  $I_b$ , respectively. After the pulse,  $I_b$  is maintained stable at a value  $I_b = I_c/2$  while the ancilla relaxes in one of its two possible states in order to measure the voltage output. If the relaxation time of the ancilla  $T_r$  is much larger than the so-called discrimination time  $T_V$  one can obtain meaningful information from a measurement and infer the qubit state<sup>8</sup>. If  $T_r$  is not long enough compared to  $T_V$ , such that a single measurement cannot provide the full information to evaluate the ancilla voltage and, consequently, the current state of flux qubit, the measurement becomes minimally invasive and weakly perturbs the quantum coherence of the evolution. An estimate of  $T_V$ , can be given by requiring that the signal-to-noise ratio approaches unity. This occurs when the spectral density  $S_V(f)$  of the output noise of the detector at fre-

quency  $f$  can be approximated as

$$S_V(f) = \lim_{\tau_m \rightarrow \infty} \frac{2|\bar{V}(f)|^2}{\tau_m} \approx \frac{2|\bar{V}(f)|^2}{T_V}. \quad (31)$$

To be more specific, let us map the values  $V = 0$  and  $V = \bar{V}$  onto a dimensionless variable  $x$  which assumes values  $\pm 1$ :  $V = \bar{V}(1+x)/2$ . Let the probability of reading a value  $x$  after the measurement  $P(x)$  be

$$P(x) = \rho_{Q\downarrow\downarrow}P_-(x) + \rho_{Q\uparrow\uparrow}P_+(x). \quad (32)$$

where  $\rho_Q$  is the reduced density matrix of the flux qubit given in Eq.(14) and  $P_{\pm}$  is the probability of having a value of  $x = \pm 1$ , as the result of the measurement.  $P_{\pm}(x)$  can be viewed as two gaussian distributions centered around  $x = \pm 1$  with the variance  $D = \frac{T_r}{T_V}$  in analogy with Ref.<sup>9</sup> where a conceptually similar approach is investigated. The change of the time of measurement in the experiment amounts to tuning the width of the  $P_{\pm}(x)$  peaks.

The Ansatz of a Gaussian distribution is due to the fact that a long measurement process gives  $V = 0$  or  $V = \bar{V}$  with probability  $\rho_{Q\downarrow\downarrow}$  or  $\rho_{Q\uparrow\uparrow}$ , while, by taking a short interaction time between qubit and ancilla, strange voltage values are not excluded<sup>10</sup>. Repeating the experiment many times, a bimodal distribution is expected with two unequal peaks centered at  $V = 0$  or  $V = \bar{V}$ , respectively.

Of course, no matter how weak the measurement is, the density matrix  $\rho_Q$  of the system turns out to be slightly modified, depending on the outcome of the measurement of the variable  $x$ . Following Ref. 11, the transformation from  $\rho_Q$  (before the measurement) to  $\rho'_Q$  (after the measurement) is defined as:

$$\begin{aligned} \rho'_{Q\downarrow\downarrow} &= \frac{\rho_{Q\downarrow\downarrow}P_-(x)}{\rho_{Q\downarrow\downarrow}P_-(x) + \rho_{Q\uparrow\uparrow}P_+(x)} \\ \rho'_{Q\downarrow\uparrow} &= \rho_{Q\downarrow\uparrow} \sqrt{\frac{\rho'_{Q\downarrow\downarrow}\rho'_{Q\uparrow\uparrow}}{\rho_{Q\downarrow\downarrow}\rho_{Q\uparrow\uparrow}}}, \quad \rho'_{Q\uparrow\downarrow} = \rho'_{Q\downarrow\uparrow}^* \\ \rho'_{Q\uparrow\uparrow} &= \frac{\rho_{Q\uparrow\uparrow}P_+(x)}{\rho_{Q\downarrow\downarrow}P_-(x) + \rho_{Q\uparrow\uparrow}P_+(x)}. \end{aligned} \quad (33)$$

This expression can be written in a more convenient form. From (33) we get

$$\frac{\rho'_{Q\downarrow\downarrow}}{\rho'_{Q\uparrow\uparrow}} = \frac{\rho_{Q\downarrow\downarrow}}{\rho_{Q\uparrow\uparrow}} \frac{P_-(x)}{P_+(x)} = \frac{\rho_{Q\downarrow\downarrow}}{\rho_{Q\uparrow\uparrow}} e^{\frac{2x}{D}}. \quad (34)$$

Let us denote with  $\gamma$  the  $x/D$  ratio and get

$$\rho'_{Q\downarrow\downarrow}\rho_{Q\uparrow\uparrow}e^{-\gamma} = \rho'_{Q\uparrow\uparrow}\rho_{Q\downarrow\downarrow}e^{\gamma}, \quad (35)$$

then

$$\rho'_{Q\downarrow\downarrow} = \frac{\rho_{Q\downarrow\downarrow}e^{\gamma}}{\rho_{Q\downarrow\downarrow}e^{\gamma} + \rho_{Q\uparrow\uparrow}e^{-\gamma}}. \quad (36)$$

Therefore, one obtains the following quantum-map from  $\rho$  to  $\rho'$ :

$$\rho'_Q = \frac{1}{\rho_{Q\downarrow\downarrow}e^{\gamma} + \rho_{Q\uparrow\uparrow}e^{-\gamma}} \begin{pmatrix} \rho_{Q\downarrow\downarrow}e^{\gamma} & \rho_{Q\downarrow\uparrow} \\ \rho_{Q\uparrow\downarrow}^* & \rho_{Q\uparrow\uparrow}e^{-\gamma} \end{pmatrix} \quad (37)$$

By tuning  $D$ , we are able to weaken the measurement till the post-measurement update in the density matrix is negligible. This is crucial if the goal is of looking at the Leggett-Garg's correlations during an annealing dynamics, without spoiling the quantum coherence of the qubit too much.

To sum up, the annealing protocol that we have realized in the simulation is the following. Firstly, one prepares the system in the ground state of the Hamiltonian  $H(0)$  and let the system evolve under  $U = e^{-iH(t/t_f)t}$ . Computationally this means solving the differential equation for the density matrix (14) with a fourth-order Runge-Kutta algorithm. At fixed times  $t_1, t_2$  (or  $t_2, t_3$  or  $t_1, t_3$ ) one performs two weak measurements, which corresponds to extracting a value of  $x$ , hence  $\sigma_z$ , from the probability distribution in Eq.(32).

To gain sufficient statistics, the same evolution is repeated several times (up to  $10^6$  times) and the Leggett-Garg's correlation functions are evaluated as an average on the different runs.

In this way, the Leggett-Garg's inequalities can be tested with weak measurements with minimal perturbation of the system during its dynamics.

The idealized measurement approach described here hides a number of experimental challenges. For a study on the back action of the detector on the flux qubit, on the problems related to the Joule heating in the dissipative state and on the fidelity of the weakness of the measurement we refer to Ref. 8 and references therein.

#### IV. GENERALIZATION TO MANY QUBITS

In this section we show how to generalize the measurement scheme in the case of many qubits. We propose to measure just one of the spins (let us say the first) while evolving (and annealing) the whole system. The hamiltonian of the system is

$$H(s) = (1-s)\frac{\Gamma_x}{2}\sum_i\sigma_x^{(i)} + s\frac{\Gamma_z}{2}\sum_i\sigma_z^{(i)} - s\sum_{i<j}J_{ij}\sigma_z^{(i)}\sigma_z^{(j)}. \quad (38)$$

We work in the computational basis, where each of the  $2^N$  states spanning the hilbert space, takes the form:

$$|\psi_i\rangle = |\sigma_z^{(1)}\sigma_z^{(2)}...\sigma_z^{(N)}\rangle_i = |\sigma_z^{(1)}\rangle_i \otimes |\sigma_z^{(2)}\rangle_i \otimes ... \otimes |\sigma_z^{(N)}\rangle_i, \quad (39)$$

where  $|\sigma_z^{(j)}\rangle_i$  is spin  $sz$  of the  $j^{th}$  particle in the  $i^{th}$  many body state. The density matrix elements are expressed as

$$\rho_{ij} = {}_i\langle\sigma_z^{(1)}\sigma_z^{(2)}...\sigma_z^{(N)}|\hat{\rho}|\sigma_z^{(1)}\sigma_z^{(2)}...\sigma_z^{(N)}\rangle_j = \langle\psi_i|\hat{\rho}|\psi_j\rangle. \quad (40)$$

As only the first spin is coupled to the detector, Eq. 32 modifies as:

$$P(x) = P_-(x)\sum_{i|\sigma_z^{(1)}=\downarrow}\rho_{ii} + P_+(x)\sum_{i|\sigma_z^{(1)}=\uparrow}\rho_{ii}. \quad (41)$$

where  $P\pm(x)$  correspond to having the two values  $x = \pm$  of the measurement depending on the up/down occupation of the first spin. The two sums are restricted to states having the first spin up or down respectively. Hence, following the same line of reasoning of the previous section, we can work out the update scheme of the density matrix from  $\rho$ , before the measurement, to  $\rho'$ , after the weak measurement:

$$\rho'_{ii} = \begin{cases} \frac{1}{P(\gamma)}\rho_{ii}e^\gamma, & \text{if } \sigma_z^{(1)} \equiv \uparrow \\ \frac{1}{P(\gamma)}\rho_{ii}e^{-\gamma}, & \text{if } \sigma_z^{(1)} \equiv \downarrow \end{cases} \quad (42)$$

and

$$\rho'_{ij} = \frac{1}{P(\gamma)}\rho_{ij} \quad (43)$$

where  $\gamma = x/D$  is defined as in in Eq.37. The correlation functions  $C_{i,j}$  necessary to evaluate the Leggett Garg functions of Eqs 25, 27, 28 are weakly measured only for the z-component of the first spin  $\sigma_z^{(1)}$ :

$$C_{i,j} = \langle\sigma_z^{(1)}(t_i)\sigma_z^{(1)}(t_j)\rangle. \quad (44)$$

This choice of the dichotomic variable is made in analogy with previous case of a simple qubit. In Fig. 3 we show a calculation of  $K_3^a$ , in the case of two qubits evolving according to Eq. 38, with  $\Gamma_x = \Gamma_z = 1$ , and for increasing values of  $J_{12} = J_{21} = J$  as a function of  $\tau = t_3 - t_2 = t_2 - t_1$  for a unitary dynamics, i.e. in the absence of coupling to the dissipative bath, performing weak measurements with  $D = 20$  and averaging over  $N = 10^6$  measurements. Increasing the exchange coupling between the two spins, the violation of LGI at the final time  $\tau = t_f/2$  is less pronounced and, for a strongly entangled system  $J/\Gamma_x > 0.4$  it no longer occurs. Such lack of violation cannot be ascribed, of course, to dissipative effects that are not included in the calculation of Fig. 3. It is better ascribed to the choice of the dichotomic variable  $\sigma_z^{(1)}$ , that does not grasp the complexity of a fully interacting system. Choosing an appropriate dichotomic variable, to maximize LGI violation at long times is a very relevant issue and will subject of further investigation. However, in order to highlight the potentiality of our technique, in what follows we will stick to  $J/\Gamma_x = 0.2$ , and turn on the system bath coupling, choosing the same parameters  $\beta = 10$ ,  $\omega_c = 25$  of the main paper, and study the evolution of the  $K_3^a$  for different values of the system bath coupling  $\alpha$ . The results are shown in Fig. 4. Even in the case of two qubits, our technique seems to be very promising, starting from maximal violation at the final time  $\tau = t_f/2$  increasing the system bath coupling  $K_3^a(t_f/2)$  gets smaller and smaller and eventually drop below the unitary limit for sizable system-bath coupling  $\alpha > 4 \cdot 10^{-3}$ . A systematic study of the multi-qubit system and its dynamics will be done elsewhere.

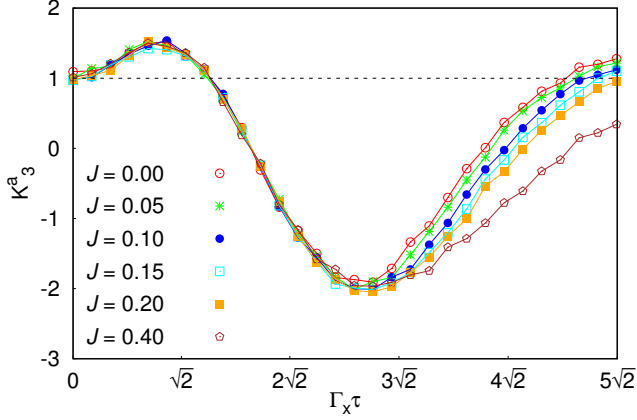

FIG. 3. Plot of the Leggett-Garg's function  $K_3^a$  during the annealing dynamics in the absence of system bath coupling for a two qubit system for different value of the exchange coupling between them (other parameters in the text). The black dashed line highlights the upper bound for the LGIs. The LG's functions are plotted as a function of the difference of the times at which the measurements are performed:  $t_2 - t_1 = t_3 - t_2 = \tau$  (in units of  $\hbar/\Gamma_x$  with  $\hbar = 1$ ). The time  $\tau$  goes from 0 to  $t_f/2$  so that it scans the whole evolution ( $t_f = 10\sqrt{2}$ ).

## V. CLASSICAL SIMULATIONS

Experimental realizations of superconducting flux qubits are based on a variable  $x$  (namely the flux) whose evolution is governed by a double well potential  $U(x)$  Ref.<sup>12</sup>. The full Hamiltonian of the system in this case is given by:

$$\hat{H} = -\frac{\hbar^2}{2m} \frac{\partial^2}{\partial x^2} + U(x), \quad (45)$$

where the mass is typically related to the device capacitance. The lowest energy states, with the variable  $x$  being confined in one of the two wells of the potential, once suitably orthogonalized correspond to the two states  $|\uparrow\rangle$  and  $|\downarrow\rangle$  of the qbit of Eq. 29. Parameters  $\Gamma_x$  and  $\Gamma_z$  are given respectively by

$$\Gamma_x = 2 \langle \downarrow | \hat{H} | \uparrow \rangle, \quad (46a)$$

$$\Gamma_z = \langle \downarrow | \hat{H} | \downarrow \rangle - \langle \uparrow | \hat{H} | \uparrow \rangle. \quad (46b)$$

Note that the wave functions corresponding to the states  $|\uparrow\rangle$  and  $|\downarrow\rangle$  always overlap to some extent, as long as the potential barrier between the wells is finite. The case  $\Gamma_z = 0$  correspond to a symmetrical double well, while  $\Gamma_x = 0$  to a very high potential barrier, so that the states do not overlap and the matrix element between them vanishes. We have devised a time dependent double well potential

$$U(x, t) = U_0 \left[ \frac{1}{4} x^4 - \frac{1}{2} a(t) x^2 - h(t) x \right], \quad (47)$$

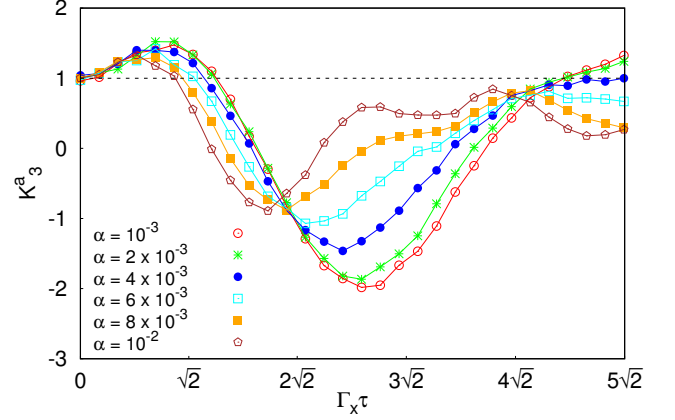

FIG. 4. Plot of the Leggett-Garg's function  $K_3^a$  during the annealing dynamics in the presence of system bath coupling with strength  $\alpha$ , for a two qubit system with the exchange coupling between them  $J/\Gamma_x = 0.2$  (other parameters in the text). The black dashed line highlights the upper bound for the LGIs. The LG's functions are plotted as a function of the difference of the times at which the measurements are performed:  $t_2 - t_1 = t_3 - t_2 = \tau$  (in units of  $\hbar/\Gamma_x$  with  $\hbar = 1$ ). The time  $\tau$  goes from 0 to  $t_f/2$  so that it scans the whole evolution ( $t_f = 10\sqrt{2}$ ).

where  $U_0$  and the functions  $a(t)$  and  $h(t)$  are chosen in the following way. We first approximate the potential near the two minima with two harmonic wells. Note that the potential has two minima as long as  $a(t)^3 > \frac{27}{4} h(t)^2$ . We then consider the two wavefunctions  $|L\rangle$  and  $|R\rangle$  corresponding to the two lowest energy states of the two harmonic wells, and orthogonalize them taking the combinations

$$|\downarrow\rangle = p|L\rangle + q|R\rangle, \quad (48a)$$

$$|\uparrow\rangle = p|R\rangle + q|L\rangle, \quad (48b)$$

where  $p$  and  $q$  are fixed by the condition that the norms are unitary and the scalar product is zero. We then impose the constraints determined by Eqs. (46), where  $\Gamma_x(t)$  and  $\Gamma_z(t)$  are given functions of the time. In particular, we choose a linear annealing procedure where  $\Gamma_x(t) = \Gamma_0 \left(1 - \frac{t}{t_f}\right)$ ,  $\Gamma_z(t) = \Gamma_0 \frac{t}{t_f}$ , where  $\Gamma_0$  is a parameter with the dimension of an energy. At time  $t = 0$ , the double well is symmetrical, so that  $h(0) = 0$ . We also set  $a(0) = x_0^2$ , so that the two minima at time zero are in  $\pm x_0$ . Note that setting the values of  $\Gamma_0$  and  $x_0$  amounts to setting the units of energy and length. For definiteness, we take  $\Gamma_0 = \hbar \nu_0$ , with  $\nu_0 = 1$  GHz. Therefore, at time zero we have two free parameters,  $U_0$  and the mass  $m$  of the particle, and only one equation, Eq. (46a), to satisfy (Eq. (46b) is satisfied being  $h(0) = 0$ ). This leaves one free parameter, that we fix imposing that the quantum ground state of the potential is higher than the barrier, and the classical oscillation frequency of the particle inside the well is equal to the Rabi frequency of

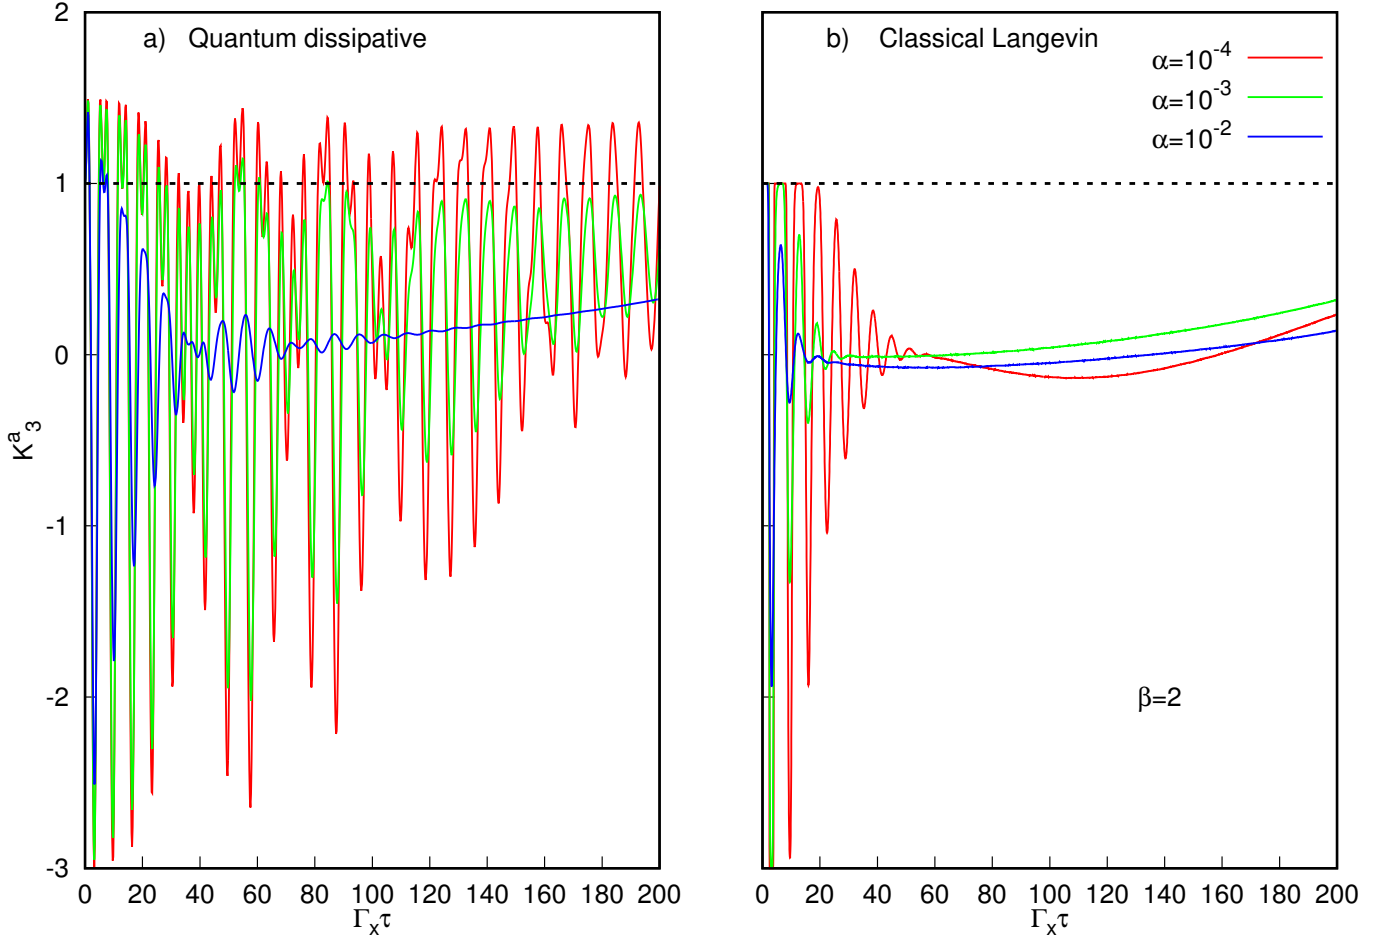

FIG. 5. Plot of the Leggett-Garg's function  $K_3^a$  during the annealing dynamics for very long annealing time  $t_f = 400$ . The black dashed line highlights the upper bound for the LGIs. The LG's functions are plotted as a function of the difference of the times at which the measurements are performed:  $t_2 - t_1 = t_3 - t_2 = \tau$  in units of  $\Gamma_x$ . The time  $\tau$  goes from 0 to  $t_f/2$  so that it scans the whole evolution ( $t_f = 400$ ). The two panels present results of quantum simulations, (panel a), and of classical Langevin dynamics (panel b). The inverse temperature is  $\beta = 2$ .

the quantum two level system, that is  $\sim 1$  GHz. For times  $t > 0$ , we leave  $U_0$  and  $m$  constant, and fix  $a(t)$  and  $h(t)$  so that the desired annealing schedule of  $\Gamma_x(t)$  and  $\Gamma_z(t)$  is realized. With time, the height of the barrier grows in order to make  $\Gamma_x(t)$  decrease, becoming much higher than the ground states of the two wells, until at time  $t = t_f$  it becomes virtually infinite (in practice we only require that  $\Gamma_x(t_f)$  is 1/1000 of the initial value, to avoid dealing with an infinite barrier).

To study the “classical analogue” of the qbit dynamics, we have simulated the classical Langevin equation

$$\ddot{x} = -\frac{1}{m} \frac{\partial U(x, t)}{\partial x} - \int_0^t \gamma(t-t') \dot{x}(t') + \xi(t), \quad (49)$$

where  $\xi(t)$  is a thermal noise with  $\langle \xi(t) \rangle = 0$  and  $\langle \xi(t) \xi(t') \rangle = \frac{k_B T}{m} \gamma(t-t')$ . We fix the function  $\gamma(t)$  postulating that Eq. (49) results from the same interaction with a thermal bath of harmonic oscillators as the spin

$\sigma_z$ , with  $x/x_0$  playing the role of  $\sigma_z$ , that is an interaction Hamiltonian

$$H_I = \frac{x}{x_0} \sum_k g_k (b_k^\dagger + b_k) + \left( \frac{x}{x_0} \right)^2 \sum_k \frac{g_k^2}{\hbar \omega_k}, \quad (50)$$

where  $b_k$  and  $b_k^\dagger$  are destruction and creation operators of oscillators with frequency  $\omega_k$ , and  $g_k$  are coupling constants with the dimensions of an energy. The second (the so called counter-) term (which is a constant when  $x/x_0$  is replaced by a spin  $\sigma_z = \pm 1$ ) ensures that the interaction with the bath does not modify the potential  $U(x, t)$  of the particle. Eliminating the bath degrees of freedom<sup>13</sup>, we obtain that the variable  $x$  obeys Eq. (49) with

$$\gamma(t) = \frac{2}{\hbar m x_0^2} \int_0^\infty d\omega \frac{J(\omega)}{\omega} \cos \omega t, \quad (51)$$

where  $J(\omega) = \sum_k g_k^2 \delta(\omega - \omega_k)$ . For an ohmic bath, consistently with Eq. 20, we set  $J(\omega) = \alpha \omega e^{-\omega/\omega_c}$ , so

that the function  $\gamma(t)$  in the limit of large  $\omega_c$  becomes the delta function  $\gamma(t) = \alpha \left( \frac{2\pi}{\hbar m x_0^2} \right) \delta(t)$ .

Comparison of classical and quantum (dissipative) dynamics are shown in Fig. 5, where we show the behaviour of the LG  $K_3^a$  functions long annealing times. A detailed discussion of the short time dynamics can be found in the main paper. In the case of long time dynamics shown in

Fig. 5, despite certain similarities, for instance in the oscillating period, the LG functions decay scales, in the two cases, are completely different. In the quantum system, notwithstanding the dissipative environment, the damping of  $K_3^a$  oscillations is much slower than the classical case for all the dissipation strength chosen.

- 
- <sup>1</sup> T. Albash, S. Boixo, D. A. Lidar, and P. Zanardi, *New Journal of Physics* **14**, 123016 (2012).
- <sup>2</sup> H. P. Breuer and F. Petruccione, *The Theory of Open Quantum Systems* (OUP Oxford, 2007).
- <sup>3</sup> A. O. Caldeira and A. J. Leggett, *Annals of Physics* **149**, 374 (1983).
- <sup>4</sup> A. J. Leggett, *Journal of Physics: Condensed Matter* **14**, R415 (2002).
- <sup>5</sup> A. J. Leggett and A. Garg, *Phys. Rev. Lett.* **54**, 857 (1985).
- <sup>6</sup> C. Emary, N. Lambert, and F. Nori, *Reports on Progress in Physics* **77**, 016001 (2014).
- <sup>7</sup> T. Picot, R. Schouten, C. Harmans, and J. Mooij, *Physical review letters* **105**, 040506 (2010).
- <sup>8</sup> A. Lupascu, C. Verwijs, R. Schouten, C. Harmans, and J. Mooij, *Physical review letters* **93**, 177006 (2004).
- <sup>9</sup> N. S. Williams and A. N. Jordan, *Phys. Rev. Lett.* **100**, 026804 (2008).
- <sup>10</sup> Y. Aharonov, D. Z. Albert, and L. Vaidman, *Phys. Rev. Lett.* **60**, 1351 (1988).
- <sup>11</sup> A. N. Jordan, A. N. Korotkov, and M. Büttiker, *Phys. Rev. Lett.* **97**, 026805 (2006).
- <sup>12</sup> R. Harris, A. J. Berkley, J. Johansson, P. Bunyk, E. M. Chapple, C. Enderud, J. P. Hilton, K. Karimi, E. Ladizinsky, N. Ladizinsky, T. Oh, I. Perminov, C. Rich, M. C. Thom, E. Tolkacheva, C. J. S. Truncik, S. Uchaikin, J. Wang, B. Wilson, and G. Rose, *Nature* **473**, 194 (2011).
- <sup>13</sup> U. Weiss, *Quantum Dissipative Systems* (World Scientific, 2012).
